# Supplementary material for: Modular implementation of the linear and cubic-scaling orbital minimization methods in electronic structure codes using atomic orbitals
Source: arXiv:2209.05934 ancillary file (2023-04-26)
Supplement: Supplementary file 1 [file SI.pdf]

# Supplementary Information for “Modular implementation of linear and cubic-scaling approaches based on the orbital minimization method in electronic structure codes using atomic orbitals”

Irina V. Lebedeva,<sup>1,2,3,\*</sup> Alberto García,<sup>4,†</sup> Emilio Artacho,<sup>1,5,6,7,‡</sup> and Pablo Ordejón<sup>2,§</sup>

<sup>1</sup>*CIC nanoGUNE BRTA, 20018 Donostia-San Sebastián, Spain*

<sup>2</sup>*Catalan Institute of Nanoscience and Nanotechnology - ICN2, CSIC and BIST, Campus UAB, 08193 Bellaterra, Spain*

<sup>3</sup>*Simune Atomistics, Avenida de Tolosa 76, 20018 Donostia-San Sebastián, Spain*

<sup>4</sup>*Institut de Ciència de Materials de Barcelona (ICMAB-CSIC), 08193 Bellaterra, Spain*

<sup>5</sup>*Donostia International Physics Center DIPC, 20018 Donostia-San Sebastián, Spain*

<sup>6</sup>*Theory of Condensed Matter, Cavendish Laboratory, University of Cambridge, Cambridge CB3 0HE, UK*

<sup>7</sup>*Ikerbasque, Basque Foundation for Science, 48011 Bilbao, Spain*

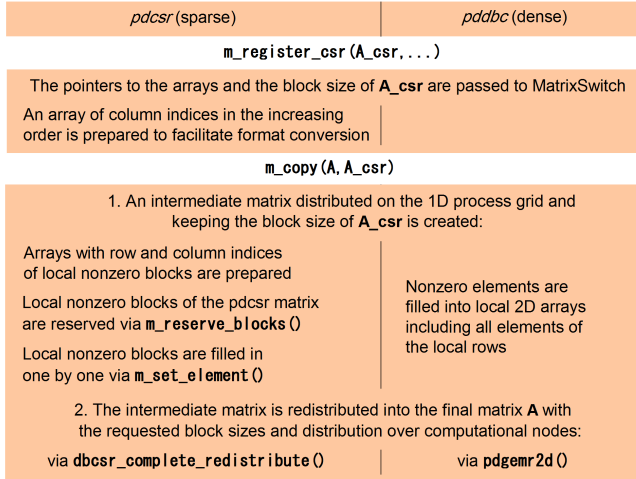

FIG. 1S. A series of calls to the MatrixSwitch library required for the format conversion of matrix **A** from the *csr* format used in SIESTA (**A\_csr**) to the *pdcsr* and *pddbc* MatrixSwitch formats (**A**) handled with the DBCSR and ScaLAPACK libraries, respectively.

## 1S. MATRIX FORMAT CONVERSION

The procedure of the format conversion of a matrix from the *csr* format used in SIESTA to the *pdcsr* and *pddbc* MatrixSwitch formats is described in Fig. 1S.

## 2S. $C^\dagger$ MATRIX INITIALIZATION AND UPDATE

The initialization of the  $C^\dagger$  matrix in the sparse form is performed in SIESTA in the following way. It is supposed that each atom carries the number of localized wavefunctions equal to the atomic charge (in units of elementary charge) divided by two,  $Q_{at}/2$ . If  $Q_{at}$  is odd,  $(Q_{at} + 1)/2$  localized wavefunctions are assigned to one atom and  $(Q_{at} - 1)/2$  to the next one. This procedure is repeated for all the atoms in the system. Then the  $C^\dagger$  matrix in the *csr* format with the total number of rows that corresponds to the total number of localized wavefunctions,  $N_{WF} = Q/2$ , where  $Q$  is the sum of atomic charges in the system, is prepared. The local rows are assigned according to the block size  $b_{WF}$  set using the input parameter **OMM.BlockSizeC**. By default, it equals the block size for the basis functions,  $b_{BF}$  (input parameter **BlockSize**), multiplied

by the ratio of the total number  $N_{WF}$  of localized wavefunctions to the basis set size  $N_{BF}$ :  $b_{WF} = b_{BF}N_{WF}/N_{BF}$ . For each local row, the local environment of the atom hosting the corresponding localized wavefunction is analyzed. The row elements that correspond to atoms beyond some cutoff radius  $R_C$  (**OMM.RcLWF**, Table 1) from the atom considered are supposed to be zero. The row elements that correspond to atoms within the cutoff radius  $R_C$  are set nonzero. This sparsity pattern is maintained during the energy functional minimization. At the beginning of the calculation run, the nonzero elements are initialized with random values. The  $C^\dagger$  matrix in the *csr* format is converted to the *pdcsr* or *pddbc* formats in the same manner as the Hamiltonian and overlap matrices, **H** and **S**.

It should be mentioned also that the initial cutoff radius  $R_C$  for initialization of the  $C^\dagger$  matrix can be set different from the one used for the energy minimization using the input parameter **OMM.RcLWFInit** (Table 1). Choosing a small initial radius (several Å) helps to avoid convergence problems both in calculations with sparse and dense matrices.

At each new MD step, the sparsity pattern of the  $C^\dagger$  matrix is checked again. The elements that now should be zero because the corresponding atoms got away by more than  $R_C$  are set to zero and no longer stored. The elements corresponding to the atoms that got closer than  $R_C$  are now stored and treated as nonzero but are assigned to zero as the initial guess. Linear extrapolation of the  $C^\dagger$  matrix based on the information from the two previous MD steps is also possible and is performed when the input parameter **OMM.Extrapolate** is set to **true** (Table 1).

## 3S. $C^\dagger$ MATRIX INPUT AND OUTPUT

The restart file for the  $C^\dagger$  matrix can be written at each SCF step (**OMM.WriteCoeffs true**, Table 1) and read at the beginning of the run (**OMM.ReadCoeffs true**). These operations are performed by calling new MS subroutines **m\_read()** and **m\_write()**, respectively (see section 6S). If the  $C^\dagger$  matrix in the *pdcsr* or *pddbc* format is distributed on a 2D process grid (**OMM.Use2D true**), it is first converted into a 1D-distributed matrix (by analogy with the format conversion routines). Then the blocks of rows are consecutively passed to the head core and written to the file. To read the file, the reverse operations are performed. The block sizes and process grid for the  $C^\dagger$  matrix do not need to be the same as used when writing the restart information. Upon reading, the sparsity pattern of the

$C^\dagger$  matrix is corrected according to the current system geometry.

#### 4S. COMPUTATIONAL DETAILS

The test calculations have been carried out for single-layer boron nitride under periodic boundary conditions. Supercells of boron nitride from  $12 \times 12$  to  $96 \times 96$  with up to 18400 atoms are considered. The lattice constant is set at 2.48 Å. The height of the simulation cell is 20 Å. The calculations have been performed at the single  $\Gamma$  point. The local density approximation,<sup>1</sup> norm-conserving Troullier-Martins<sup>2</sup> pseudopotentials and standard built-in DZP basis set<sup>3</sup> are used. The atomic orbitals are set to zero beyond the cutoff determined by the energy shift of 10 meV (cutoff radii 2.5 – 4.5 Å). The real-space grid is equivalent to the plane-wave cutoff energy of 100 Ry. The linear mixing scheme with a mixing parameter of 0.1 is applied to converge the ground state. The tolerance is  $10^{-4}$  for the density matrix and  $10^{-3}$  eV for the matrix elements of the Hamiltonian.

To test performance of different approaches in MD simulations, several MD steps starting from the converged ground state have been computed (the ground state is converged previously with the same method as used for MD). The microcanonical ensemble with an initial temperature of 300 K is considered. The Verlet algorithm<sup>4</sup> with a time step of 1 fs is used. The Pulay mixing scheme<sup>5</sup> with a mixing parameter of 0.2 is applied during the MD simulations.

The matrices involved in the calculations consist of equal blocks. For the DZP basis set, each boron and nitrogen atom has 13 basis functions, and hosts 3 or 2 wavefunctions depending on whether the unoccupied states are included into consideration or not, respectively. Therefore, the block size for the wavefunctions is usually chosen to be  $b_{WF} = 6$  (input parameter `OMM.BlockSizeC`, Table 1) and for the basis functions  $b_{BF} = 13$  (input parameter `BlockSize`). The matrices are distributed on a 2D process grid (`OMM.Use2D true`). The cutoff radius for localized wavefunctions (`OMM.RcLWF`) in typical calculations with sparse matrices is  $R_C = 4$  Å. The chemical potential for the Kim functional (`OMM.Eta`) is  $\eta = -5.5$  eV. CG iterations are performed until the difference of energies at consecutive CG iterations divided by the average energy at these iterations (`OMM.RelTol`) reaches  $10^{-9}$ . The tests with the preconditioning for dense matrices have been carried out using the scale for the kinetic energy of  $\tau_T = 10$  Ry (Ref. 6).

#### 5S. CUTOFF RADIUS EFFECT ON CALCULATION RESULTS

In Fig. 2S, we address the accuracy of force and energy calculations with the Ordejón-Mauri and Kim methods. The deviation from the results for the wavefunctions without localization ( $R_C \rightarrow \infty$ ) is plotted for different cutoff radii  $R_C$ . It is seen that for both of the methods, the accuracy improves upon increasing the cutoff radius in a similar manner. The deviations of the energy and forces within 10 meV/atom and 0.02 eV/Å are achieved already for the cutoff radius of  $R_C = 4$  Å, in agreement with previous publications.<sup>7,8</sup> Therefore, to reach

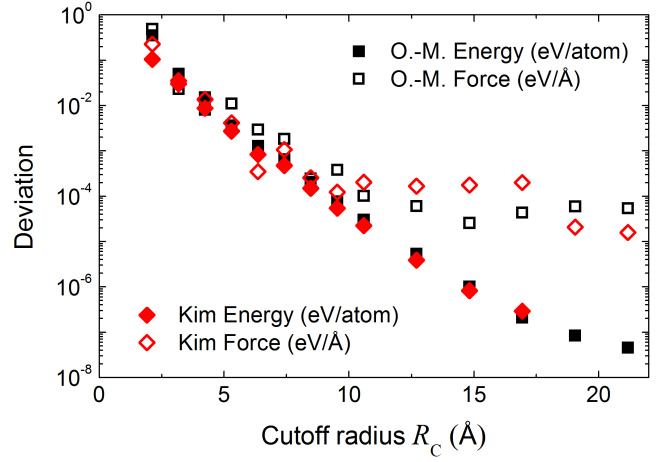

FIG. 2S. Deviations of energy (in eV/atom, closed symbols) and force (in eV/Å, open symbols) for the  $60 \times 60$  supercell of boron nitride (7200 atoms) with atoms displaced by 0.05 Å from their equilibrium positions from the results for the infinite cutoff radius for the wavefunctions  $R_C \rightarrow \infty$  vs cutoff radius  $R_C$  (in Å): (black squares) Ordejón-Mauri and (red diamonds) Kim methods. A double-zeta polarized basis set is used. The chemical potential for the Kim method is  $\eta = -5.5$  eV. The block size is  $b_{WF} = 6$  for the localized wavefunctions and  $b_{BF} = 13$  for the basis functions.

the chemical accuracy, it is sufficient to consider cutoff radii of several Å.

#### 6S. MATRIXSWITCH OVERVIEW

As discussed in the main text, several changes to the MS library have been introduced to implement the OMM solver such as the extension of the subroutines for the matrix format conversion, addition of subroutines for matrix reading and writing, etc. Let us, therefore, give a short overview of the current capabilities of the MS library for operations with sparse matrices in the *pdcsr* format using the DBCSR library and dense matrices in the *pddbc* format using the ScaLAPACK library (Tables 1S, 2S, 3S and 4S).

First `ms_dbcsr_setup()` or `ms_scalapack_setup()` should be called to initialize the DBCSR or ScaLAPACK library, respectively, and set up the process grid used to store the matrix elements (Table 1S). Matrices can be allocated using `m_allocate()` specifying the matrix dimensions, block sizes for rows and columns or arrays of block sizes (if non-equal blocks are used) and deallocated using `m_deallocate()`. If local 2D arrays of elements of a dense matrix are already prepared, the matrix can be registered in the *pddbc* format through `m_register_pdbc()`. Also the pointers to the arrays of a *csr* matrix can be passed to MS via `m_register_csr()`. Although algebraic operations for this matrix format are not defined in MS, *csr* matrices can be converted to the *pdcsr* or *pddbc* format.

The elements of *pdcsr* or *pddbc* matrices can be filled in using `m_set_element()` and `m_set()` (Table 2S). The subroutine `m_set_element()` allows to set a *pddbc* matrix element by element or a *pdcsr* matrix block by block. In the case of

*pdcsr* matrices, nonempty blocks can be reserved providing their row and column indices via `m_reserve_blocks()`. This subroutine should be called before setting the matrix elements to achieve linear scaling. The subroutine `m_set()` can be used to assign different values to diagonal and non-diagonal elements. However, in the case of a *pdcsr* matrix only diagonal elements can be set in this way (otherwise, the matrix will no longer be sparse). The information on the matrix elements can be retrieved using `m_get_element()`. Again, in the case of sparse matrices in the *pdcsr* format, a 2D array corresponding to a single block is obtained in this way. The occupation of a *pdcsr* matrix, i.e. the fraction of nonempty elements, can be found using `m_occupation()`.

Algebraic operations for matrices such as addition, multiplication, scaling, calculation of trace are performed using calls to `m_add()`, `mm_multiply()`, `m_scale()`, `mm_trace()` and `m_trace()`, respectively (Table 3S). Note that it can be specified whether the operations should be performed on the matrix as it is or on its transpose or Hermitian conjugate.

Writing and reading of *pdcsr* and *pddbc* matrices is carried out using the subroutines `m_read()` and `m_write()` (Table 4S). An exact copy of a matrix can be created using `m_copy()`. However, if the target matrix where the data are filled in is already allocated before calling the subroutine, only values of the matrix elements are copied into it. In the case of the *pdcsr* format, the sparsity pattern of the target matrix is maintained. That is matrix elements that are empty are kept empty, although they can be nonempty in the source matrix. The nonempty elements that are empty in the source matrix are set to zero. If the target matrix has a format different from that of the source matrix, the conversion of the matrix format takes place. In this way, a *csr* matrix can be converted into a *pdcsr* or *pddbc* one or vice versa. An intermediate matrix `m_sp` with the same distribution of rows over the CPU cores as the *csr* matrix can be provided. If it is allocated before calling the subroutine, its sparsity pattern is maintained during the conversion.

---

\* liv.ira@hotmail.com

† albertog@icmab.es

‡ ea245@cam.ac.uk

§ pablo.ordejón@icn2.cat

<sup>1</sup> J. P. Perdew and A. Zunger, Phys. Rev. B **23**, 5048 (1981).

<sup>2</sup> N. Troullier and J. L. Martins, Phys. Rev. B **43**, 1993 (1991).

<sup>3</sup> J. Junquera, O. Paz, D. Sánchez-Portal, and E. Artacho, Phys. Rev. B **64**, 235111 (2001).

<sup>4</sup> M. P. Allen and D. J. Tildesley, *Computer Simulation of Liquids* (Oxford: Oxford University Press, 1987).

<sup>5</sup> G. Kresse and J. Furthmüller, Comput. Mater. Sci. **6**, 15 (1996).

<sup>6</sup> F. Corsetti, Computer Physics Communications **185**, 873 (2014).

<sup>7</sup> P. Ordejón, D. A. Drabold, R. M. Martin, and M. P. Grumbach, Phys. Rev. B **51**, 1456 (1995).

<sup>8</sup> F. Mauri and G. Galli, Phys. Rev. B **50**, 4316 (1994).

TABLE 1S. The public subroutines of the MatrixSwitch library for the calculation setup, creation and destruction of *pdcscr*, *pddbc*<sup>a</sup> and *csr* matrices.

| Parameter                                                                                                                                                                                                                                                                                                            | Input/Output    | Type                         | Description                                                                                                                                                                                                                                               |
|----------------------------------------------------------------------------------------------------------------------------------------------------------------------------------------------------------------------------------------------------------------------------------------------------------------------|-----------------|------------------------------|-----------------------------------------------------------------------------------------------------------------------------------------------------------------------------------------------------------------------------------------------------------|
| <b>ms_dbcsr_setup(mpi_comm, bs_def, use2D)</b>                                                                                                                                                                                                                                                                       |                 |                              |                                                                                                                                                                                                                                                           |
| Sets up everything needed to use <i>pdcscr</i> matrices with the DBCSR library. Should be called once at the beginning of the code.                                                                                                                                                                                  |                 |                              |                                                                                                                                                                                                                                                           |
| <b>mpi_comm</b>                                                                                                                                                                                                                                                                                                      | input           | integer                      | The MPI communicator to use                                                                                                                                                                                                                               |
| <b>bs_def</b>                                                                                                                                                                                                                                                                                                        | input           | integer                      | The default block size for matrices                                                                                                                                                                                                                       |
| <b>use2D</b>                                                                                                                                                                                                                                                                                                         | input, optional | logical                      | Whether to use a 2D process grid by default                                                                                                                                                                                                               |
| <b>ms_dbcsr_finalize()</b>                                                                                                                                                                                                                                                                                           |                 |                              |                                                                                                                                                                                                                                                           |
| Finalizes the use of the DBCSR library. Should be called once at the end of the code.                                                                                                                                                                                                                                |                 |                              |                                                                                                                                                                                                                                                           |
| <b>ms_scalapack_setup(mpi_comm, nprow, order, bs_def, bs_list, icontxt, icontxt_1D)</b>                                                                                                                                                                                                                              |                 |                              |                                                                                                                                                                                                                                                           |
| Sets up everything needed to use <i>pddbc</i> matrices with the ScaLAPACK library. Should be called once at the beginning of the code.                                                                                                                                                                               |                 |                              |                                                                                                                                                                                                                                                           |
| <b>mpi_comm</b>                                                                                                                                                                                                                                                                                                      | input           | integer                      | The MPI communicator to use                                                                                                                                                                                                                               |
| <b>nrow</b>                                                                                                                                                                                                                                                                                                          | input           | integer                      | The row dimension of the process grid                                                                                                                                                                                                                     |
| <b>order</b>                                                                                                                                                                                                                                                                                                         | input           | character(1)                 | The ordering of the process grid (c/C: column-major, r/R: row-major)                                                                                                                                                                                      |
| <b>bs_def</b>                                                                                                                                                                                                                                                                                                        | input           | integer                      | The default block size for matrices                                                                                                                                                                                                                       |
| <b>bs_list</b>                                                                                                                                                                                                                                                                                                       | input, optional | integer, 1D array            | The list of exceptions to <b>bs_def</b> for specific matrix sizes formatted as <b>dim<sub>1</sub>, bs<sub>1</sub>, dim<sub>2</sub>, bs<sub>2</sub>, etc.</b> , where <b>bs<sub>n</sub></b> is the block size for dimension of size <b>dim<sub>n</sub></b> |
| <b>icontxt</b>                                                                                                                                                                                                                                                                                                       | input, optional | integer                      | The BLACS context handle                                                                                                                                                                                                                                  |
| <b>icontxt_1D</b>                                                                                                                                                                                                                                                                                                    | input, optional | integer                      | The BLACS context handle for the 1D process grid                                                                                                                                                                                                          |
| <b>m_allocate(m_name, dim1, dim2, label, use2D, blocksize1, blocksize2, row_sizes, col_sizes)</b>                                                                                                                                                                                                                    |                 |                              |                                                                                                                                                                                                                                                           |
| Initializes a matrix of the <i>pdcscr</i> , <i>pddbc</i> or other format by saving the basic information (dimensions, block sizes, shape, type of elements, etc.). The matrix elements are set zero or empty if the matrix format is <i>pdcscr</i> . If the block sizes are not provided, the default value is used. |                 |                              |                                                                                                                                                                                                                                                           |
| <b>m_name</b>                                                                                                                                                                                                                                                                                                        | input/output    | type(matrix)                 | The matrix to be allocated                                                                                                                                                                                                                                |
| <b>dim1</b>                                                                                                                                                                                                                                                                                                          | input           | integer                      | The number of rows in the matrix                                                                                                                                                                                                                          |
| <b>dim2</b>                                                                                                                                                                                                                                                                                                          | input           | integer                      | The number of columns in the matrix                                                                                                                                                                                                                       |
| <b>label</b>                                                                                                                                                                                                                                                                                                         | input, optional | character(5)                 | The storage format to use                                                                                                                                                                                                                                 |
| <b>use2D</b>                                                                                                                                                                                                                                                                                                         | input, optional | logical                      | Whether to use a 2D process grid                                                                                                                                                                                                                          |
| <b>blocksize1</b>                                                                                                                                                                                                                                                                                                    | input, optional | integer                      | The block size for rows (if equal)                                                                                                                                                                                                                        |
| <b>blocksize2</b>                                                                                                                                                                                                                                                                                                    | input, optional | integer                      | The block size for columns (if equal)                                                                                                                                                                                                                     |
| <b>row_sizes</b>                                                                                                                                                                                                                                                                                                     | input, optional | integer, pointer, 1D array   | The block sizes for rows                                                                                                                                                                                                                                  |
| <b>col_sizes</b>                                                                                                                                                                                                                                                                                                     | input, optional | integer, pointer, 1D array   | The block sizes for columns                                                                                                                                                                                                                               |
| <b>m_deallocate(m_name)</b>                                                                                                                                                                                                                                                                                          |                 |                              |                                                                                                                                                                                                                                                           |
| Deallocates all the arrays allocated. Nullifies all the pointers.                                                                                                                                                                                                                                                    |                 |                              |                                                                                                                                                                                                                                                           |
| <b>m_name</b>                                                                                                                                                                                                                                                                                                        | input/output    | type(matrix)                 | The matrix to be deallocated                                                                                                                                                                                                                              |
| <b>m_register_csr(m_name, dim1, dim2, nrow, id_rows, id_cols, nze_row, val, ind_ordered, order, blk_size)</b>                                                                                                                                                                                                        |                 |                              |                                                                                                                                                                                                                                                           |
| Passes the pointers to the arrays of the <i>csr</i> matrix to MatrixSwitch. Orders the elements in such a way that column indices for each row are arranged in the growing order.                                                                                                                                    |                 |                              |                                                                                                                                                                                                                                                           |
| <b>m_name</b>                                                                                                                                                                                                                                                                                                        | input/output    | type(matrix)                 | The <i>csr</i> matrix to be registered                                                                                                                                                                                                                    |
| <b>dim1</b>                                                                                                                                                                                                                                                                                                          | input           | integer                      | The number of rows                                                                                                                                                                                                                                        |
| <b>dim2</b>                                                                                                                                                                                                                                                                                                          | input           | integer                      | The number of columns                                                                                                                                                                                                                                     |
| <b>nrow</b>                                                                                                                                                                                                                                                                                                          | input           | integer                      | The number of local rows                                                                                                                                                                                                                                  |
| <b>id_rows</b>                                                                                                                                                                                                                                                                                                       | input           | integer, 1D array            | The indices of the start of local rows                                                                                                                                                                                                                    |
| <b>id_cols</b>                                                                                                                                                                                                                                                                                                       | input           | integer, 1D array            | The column indices of nonempty matrix elements of the local rows                                                                                                                                                                                          |
| <b>nze_row</b>                                                                                                                                                                                                                                                                                                       | input           | integer, 1D array            | The number of nonempty matrix elements in each local row                                                                                                                                                                                                  |
| <b>val</b>                                                                                                                                                                                                                                                                                                           | input           | integer, 1D array            | The values of nonempty matrix elements in the local rows                                                                                                                                                                                                  |
| <b>ind_ordered</b>                                                                                                                                                                                                                                                                                                   | input, optional | integer, 1D array            | The indices ordered in such a way that the column indices of each row become ordered                                                                                                                                                                      |
| <b>order</b>                                                                                                                                                                                                                                                                                                         | input, optional | logical                      | Whether to order the indices                                                                                                                                                                                                                              |
| <b>blk_size</b>                                                                                                                                                                                                                                                                                                      | input, optional | integer                      | The block size for the rows. If not provided, the default value is used                                                                                                                                                                                   |
| <b>m_register_pdbc(m_name, A, desc)</b>                                                                                                                                                                                                                                                                              |                 |                              |                                                                                                                                                                                                                                                           |
| Passes the pointers to the local 2D arrays to MatrixSwitch to register them as a <i>pddbc</i> matrix                                                                                                                                                                                                                 |                 |                              |                                                                                                                                                                                                                                                           |
| <b>m_name</b>                                                                                                                                                                                                                                                                                                        | input/output    | type(matrix)                 | The <i>pddbc</i> matrix to be registered                                                                                                                                                                                                                  |
| <b>A</b>                                                                                                                                                                                                                                                                                                             | input           | real <sup>b</sup> , 2D array | The 2D array with local matrix elements                                                                                                                                                                                                                   |
| <b>desc</b>                                                                                                                                                                                                                                                                                                          | input           | integer, 1D array(9)         | The BLACS descriptor                                                                                                                                                                                                                                      |

<sup>a</sup> The same subroutines can be also used for matrices in the *pzdbc* format, which is a complex analogue of *pddbc*.

<sup>b</sup> Double precision (or complex(16) for *pzdbc* matrices).

TABLE 2S. The public subroutines of the MatrixSwitch library for manipulation of the data stored in *pdcsr* and *pddbc*<sup>a</sup> matrices.

| Parameter                                                                                                                                                                                                                                                                                                                          | Input/Output    | Type                                                                                 | Description                                                                                                      |
|------------------------------------------------------------------------------------------------------------------------------------------------------------------------------------------------------------------------------------------------------------------------------------------------------------------------------------|-----------------|--------------------------------------------------------------------------------------|------------------------------------------------------------------------------------------------------------------|
| <b>m_set_element(C, i, j, alpha, beta, label)</b>                                                                                                                                                                                                                                                                                  |                 |                                                                                      |                                                                                                                  |
| Changes an element of a dense matrix <b>C</b> (e.g., <i>pddbc</i> ) or a 2D block for a <i>pdcsr</i> matrix <b>C</b> with indices <i>i</i> and <i>j</i> as follows: $C_{ij} = \alpha + \beta C_{ij}$ .                                                                                                                             |                 |                                                                                      |                                                                                                                  |
| <b>C</b>                                                                                                                                                                                                                                                                                                                           | input/output    | type(matrix)                                                                         | The matrix in which the element (block) is set                                                                   |
| <b>i</b>                                                                                                                                                                                                                                                                                                                           | input           | integer                                                                              | The row index of the element (block)                                                                             |
| <b>j</b>                                                                                                                                                                                                                                                                                                                           | input           | integer                                                                              | The column index of the element (block)                                                                          |
| <b>alpha</b>                                                                                                                                                                                                                                                                                                                       | input           | real <sup>b</sup> (for a dense matrix)<br>real, 2D array (for a <i>pdcsr</i> matrix) | The value $\alpha$ to be set<br>The 2D block $\alpha$ to be set                                                  |
| <b>beta</b>                                                                                                                                                                                                                                                                                                                        | input           | real <sup>b</sup>                                                                    | The coefficient $\beta$ for the operation described above                                                        |
| <b>label</b>                                                                                                                                                                                                                                                                                                                       | input, optional | character(3)                                                                         | The implementation of the operation to use <sup>c</sup>                                                          |
| <b>m_set(C, seC, alpha, beta, label)</b>                                                                                                                                                                                                                                                                                           |                 |                                                                                      |                                                                                                                  |
| Sets diagonal elements of a matrix <b>C</b> to $\beta$ ( $C_{ij} = \beta$ for $i = j$ ) and non-diagonal to $\alpha$ ( $C_{ij} = \alpha$ for $i \neq j$ ). For the <i>pddbc</i> and other dense formats, it is possible to assign the values only to the lower/upper triangle (below/above the diagonal for rectangular matrices). |                 |                                                                                      |                                                                                                                  |
| <b>C</b>                                                                                                                                                                                                                                                                                                                           | input/output    | type(matrix)                                                                         | The matrix in which the element is set                                                                           |
| <b>seC</b>                                                                                                                                                                                                                                                                                                                         | input           | character(1)                                                                         | The form of the operation: l/L - lower triangle, u/U - upper triangle, other - complete matrix                   |
| <b>alpha</b>                                                                                                                                                                                                                                                                                                                       | input           | real <sup>b</sup>                                                                    | The value $\alpha$ to be set                                                                                     |
| <b>beta</b>                                                                                                                                                                                                                                                                                                                        | input           | real <sup>b</sup>                                                                    | The value $\beta$ to be set                                                                                      |
| <b>label</b>                                                                                                                                                                                                                                                                                                                       | input, optional | character(3)                                                                         | The implementation of the operation to use <sup>c</sup>                                                          |
| <b>m_get_element(C, i, j, alpha, label, found)</b>                                                                                                                                                                                                                                                                                 |                 |                                                                                      |                                                                                                                  |
| Performs the operation: $\alpha = C_{ij}$ , where $C_{ij}$ is a matrix element of a dense matrix <b>C</b> (e.g., <i>pddbc</i> ) or a 2D block of a <i>pdcsr</i> matrix <b>C</b> .                                                                                                                                                  |                 |                                                                                      |                                                                                                                  |
| <b>C</b>                                                                                                                                                                                                                                                                                                                           | input           | type(matrix)                                                                         | The matrix considered                                                                                            |
| <b>i</b>                                                                                                                                                                                                                                                                                                                           | input           | integer                                                                              | The row index of the element (block)                                                                             |
| <b>j</b>                                                                                                                                                                                                                                                                                                                           | input           | integer                                                                              | The column index of the element (block)                                                                          |
| <b>alpha</b>                                                                                                                                                                                                                                                                                                                       | output          | real <sup>b</sup> (for a dense matrix)<br>real, 2D array (for a <i>pdcsr</i> matrix) | The scalar $\alpha$ for the operation described above<br>The 2D block $\alpha$ for the operation described above |
| <b>label</b>                                                                                                                                                                                                                                                                                                                       | input, optional | character(3)                                                                         | The implementation of the operation to use <sup>c</sup>                                                          |
| <b>found</b>                                                                                                                                                                                                                                                                                                                       | output          | logical                                                                              | Whether the block is found                                                                                       |
| <b>m_reserve_blocks(C, rows, cols)</b>                                                                                                                                                                                                                                                                                             |                 |                                                                                      |                                                                                                                  |
| Reserves nonempty blocks of a <i>pdcsr</i> matrix.                                                                                                                                                                                                                                                                                 |                 |                                                                                      |                                                                                                                  |
| <b>C</b>                                                                                                                                                                                                                                                                                                                           | input/output    | type(matrix)                                                                         | The matrix to be filled in                                                                                       |
| <b>rows</b>                                                                                                                                                                                                                                                                                                                        | input           | integer, 1D array                                                                    | The row indices of nonempty blocks                                                                               |
| <b>cols</b>                                                                                                                                                                                                                                                                                                                        | input           | integer, 1D array                                                                    | The column indices of nonempty blocks                                                                            |
| <b>m_occupation(C, occ)</b>                                                                                                                                                                                                                                                                                                        |                 |                                                                                      |                                                                                                                  |
| Calculates the fraction of nonempty blocks (i.e. occupation) of a <i>pdcsr</i> matrix.                                                                                                                                                                                                                                             |                 |                                                                                      |                                                                                                                  |
| <b>C</b>                                                                                                                                                                                                                                                                                                                           | input/output    | type(matrix)                                                                         | The matrix analyzed                                                                                              |
| <b>occ</b>                                                                                                                                                                                                                                                                                                                         | output          | real                                                                                 | The occupation found                                                                                             |

<sup>a</sup> The same subroutines can be also used for matrices in the *pzdbc* format, which is a complex analogue of *pddbc*.<sup>b</sup> Double precision (or complex(16) for *pzdbc* matrices).<sup>c</sup> For *pdcsr* and *pddbc* matrices, should be set to 'lap' (external linear algebra libraries are used) or omitted.

TABLE 3S. The public subroutines of the MatrixSwitch library for algebraic operations with matrices.

| Parameter                                                                                                                                                                                                                  | Input/Output    | Type              | Description                                                                                                               |
|----------------------------------------------------------------------------------------------------------------------------------------------------------------------------------------------------------------------------|-----------------|-------------------|---------------------------------------------------------------------------------------------------------------------------|
| <b>mm_multiply(A, opA, B, opB, C, alpha, beta, label, keep_sparsity)</b>                                                                                                                                                   |                 |                   |                                                                                                                           |
| For matrices <b>A</b> , <b>B</b> and <b>C</b> , performs the operation $C = \alpha \tilde{A}\tilde{B} + \beta C$ . Here $\tilde{M}$ can be <b>M</b> , the transposed matrix $M^T$ or the Hermitian conjugate $M^\dagger$ . |                 |                   |                                                                                                                           |
| <b>A</b>                                                                                                                                                                                                                   | input           | type(matrix)      | The matrix <b>A</b>                                                                                                       |
| <b>opA</b>                                                                                                                                                                                                                 | input           | character(1)      | The form of <b>A</b> : n/N - normal ( <b>A</b> ), t/T - transposed ( $A^T$ )<br>c/C - Hermitian conjugate ( $A^\dagger$ ) |
| <b>B</b>                                                                                                                                                                                                                   | input           | type(matrix)      | The matrix <b>B</b>                                                                                                       |
| <b>opB</b>                                                                                                                                                                                                                 | input           | character(1)      | The form of <b>B</b>                                                                                                      |
| <b>C</b>                                                                                                                                                                                                                   | input/output    | type(matrix)      | The matrix <b>C</b>                                                                                                       |
| <b>alpha</b>                                                                                                                                                                                                               | input           | real <sup>a</sup> | The coefficient $\alpha$                                                                                                  |
| <b>beta</b>                                                                                                                                                                                                                | input           | real <sup>a</sup> | The coefficient $\beta$                                                                                                   |
| <b>label</b>                                                                                                                                                                                                               | input, optional | character(3)      | The implementation of the operation to use <sup>b</sup>                                                                   |
| <b>keep_sparsity</b>                                                                                                                                                                                                       | input, optional | logical           | Whether to maintain sparsity of matrix <b>C</b>                                                                           |
| <b>m_add(A, opA, C, alpha, beta, label)</b>                                                                                                                                                                                |                 |                   |                                                                                                                           |
| For matrices <b>A</b> and <b>C</b> , performs the operation $C = \alpha \tilde{A} + \beta C$ . Here $\tilde{M}$ can be <b>M</b> , the transposed matrix $M^T$ or the Hermitian conjugate $M^\dagger$ .                     |                 |                   |                                                                                                                           |
| <b>A</b>                                                                                                                                                                                                                   | input           | type(matrix)      | The matrix <b>A</b>                                                                                                       |
| <b>opA</b>                                                                                                                                                                                                                 | input           | character(1)      | The form of <b>A</b> : n/N - normal ( <b>A</b> ), t/T - transposed ( $A^T$ )<br>c/C - Hermitian conjugate ( $A^\dagger$ ) |
| <b>C</b>                                                                                                                                                                                                                   | input/output    | type(matrix)      | The matrix <b>C</b>                                                                                                       |
| <b>alpha</b>                                                                                                                                                                                                               | input           | real <sup>a</sup> | The coefficient $\alpha$                                                                                                  |
| <b>beta</b>                                                                                                                                                                                                                | input           | real <sup>a</sup> | The coefficient $\beta$                                                                                                   |
| <b>label</b>                                                                                                                                                                                                               | input, optional | character(3)      | The implementation of the operation to use <sup>b</sup>                                                                   |
| <b>mm_trace(A, B, alpha, label)</b>                                                                                                                                                                                        |                 |                   |                                                                                                                           |
| For matrices <b>A</b> and <b>B</b> , performs the operation $\alpha = \text{Tr}[\tilde{A}B]$ .                                                                                                                             |                 |                   |                                                                                                                           |
| <b>A</b>                                                                                                                                                                                                                   | input           | type(matrix)      | The matrix <b>A</b>                                                                                                       |
| <b>B</b>                                                                                                                                                                                                                   | input           | type(matrix)      | The matrix <b>B</b>                                                                                                       |
| <b>alpha</b>                                                                                                                                                                                                               | output          | real <sup>a</sup> | The trace computed                                                                                                        |
| <b>label</b>                                                                                                                                                                                                               | input, optional | character(3)      | The implementation of the operation to use <sup>b</sup>                                                                   |
| <b>m_trace(A, alpha, label)</b>                                                                                                                                                                                            |                 |                   |                                                                                                                           |
| For a matrix <b>A</b> , performs the operation $\alpha = \text{Tr}[\tilde{A}]$ .                                                                                                                                           |                 |                   |                                                                                                                           |
| <b>A</b>                                                                                                                                                                                                                   | input           | type(matrix)      | The matrix <b>A</b>                                                                                                       |
| <b>alpha</b>                                                                                                                                                                                                               | output          | real <sup>a</sup> | The trace computed                                                                                                        |
| <b>label</b>                                                                                                                                                                                                               | input, optional | character(3)      | The implementation of the operation to use <sup>b</sup>                                                                   |
| <b>m_scale(C, beta, label)</b>                                                                                                                                                                                             |                 |                   |                                                                                                                           |
| For a matrix <b>C</b> , performs the operation $C = \beta C$ .                                                                                                                                                             |                 |                   |                                                                                                                           |
| <b>C</b>                                                                                                                                                                                                                   | input/output    | type(matrix)      | The matrix <b>C</b>                                                                                                       |
| <b>beta</b>                                                                                                                                                                                                                | output          | real <sup>a</sup> | The scaling coefficient $\beta$                                                                                           |
| <b>label</b>                                                                                                                                                                                                               | input, optional | character(3)      | The implementation of the operation to use <sup>b</sup>                                                                   |

<sup>a</sup> Double precision (or complex(16) for complex matrices like *pzdbc*).<sup>b</sup> For *pdcsr* and *pddbc* matrices, should be set to 'lap' (external linear algebra libraries are used) or omitted.

TABLE 4S. The public subroutines of the MatrixSwitch library for reading, writing and copying of *pdcsr* and *pddbc* matrices.

| Parameter                                                                                                                                                                                                                                                                                                                                                                                                                                                                                                                                                                                                                                                                                                                                    | Input/Output     | Type         | Description                                                                                                                                                                 |
|----------------------------------------------------------------------------------------------------------------------------------------------------------------------------------------------------------------------------------------------------------------------------------------------------------------------------------------------------------------------------------------------------------------------------------------------------------------------------------------------------------------------------------------------------------------------------------------------------------------------------------------------------------------------------------------------------------------------------------------------|------------------|--------------|-----------------------------------------------------------------------------------------------------------------------------------------------------------------------------|
| <b>m_read(m_name,filepath,file_exist,keep_sparsity,use_dbcsrlib,nze)</b>                                                                                                                                                                                                                                                                                                                                                                                                                                                                                                                                                                                                                                                                     |                  |              |                                                                                                                                                                             |
| Reads a <i>pdcsr</i> or <i>pddbc</i> matrix from the file. The new dimensions, block sizes and process grid can be different.                                                                                                                                                                                                                                                                                                                                                                                                                                                                                                                                                                                                                |                  |              |                                                                                                                                                                             |
| m_name                                                                                                                                                                                                                                                                                                                                                                                                                                                                                                                                                                                                                                                                                                                                       | input/output     | type(matrix) | The matrix to be read                                                                                                                                                       |
| filepath                                                                                                                                                                                                                                                                                                                                                                                                                                                                                                                                                                                                                                                                                                                                     | input            | character    | The path to the file                                                                                                                                                        |
| file_exist                                                                                                                                                                                                                                                                                                                                                                                                                                                                                                                                                                                                                                                                                                                                   | output           | logical      | Whether the file is found                                                                                                                                                   |
| keep_sparsity                                                                                                                                                                                                                                                                                                                                                                                                                                                                                                                                                                                                                                                                                                                                | input, optional  | logical      | Whether to use sparsity of the input matrix (for <i>pdcsr</i> matrices)                                                                                                     |
| use_dbcsrlib                                                                                                                                                                                                                                                                                                                                                                                                                                                                                                                                                                                                                                                                                                                                 | input, optional  | logical      | Whether to use the DBCSR library for reading (for <i>pdcsr</i> matrices)                                                                                                    |
| nze                                                                                                                                                                                                                                                                                                                                                                                                                                                                                                                                                                                                                                                                                                                                          | input, optional  | integer      | An expected number of local nonzero elements in the intermediate matrix distributed on the 1D process grid (for <i>pdcsr</i> matrices)                                      |
| <b>m_write(m_name,filepath,use_dbcsrlib,nze)</b>                                                                                                                                                                                                                                                                                                                                                                                                                                                                                                                                                                                                                                                                                             |                  |              |                                                                                                                                                                             |
| Writes a <i>pdcsr</i> or <i>pddbc</i> matrix to the file.                                                                                                                                                                                                                                                                                                                                                                                                                                                                                                                                                                                                                                                                                    |                  |              |                                                                                                                                                                             |
| m_name                                                                                                                                                                                                                                                                                                                                                                                                                                                                                                                                                                                                                                                                                                                                       | input/output     | type(matrix) | The matrix to be written                                                                                                                                                    |
| filepath                                                                                                                                                                                                                                                                                                                                                                                                                                                                                                                                                                                                                                                                                                                                     | input            | character    | The path to the file                                                                                                                                                        |
| use_dbcsrlib                                                                                                                                                                                                                                                                                                                                                                                                                                                                                                                                                                                                                                                                                                                                 | input, optional  | logical      | Whether to use the DBCSR library for writing (for <i>pdcsr</i> matrices)                                                                                                    |
| nze                                                                                                                                                                                                                                                                                                                                                                                                                                                                                                                                                                                                                                                                                                                                          | input, optional  | integer      | An expected number of local nonzero elements in the intermediate matrix distributed on the 1D process grid (for <i>pdcsr</i> matrices)                                      |
| <b>m_copy(m_name,A,label,threshold,threshold_is_soft,m_sp)</b>                                                                                                                                                                                                                                                                                                                                                                                                                                                                                                                                                                                                                                                                               |                  |              |                                                                                                                                                                             |
| Copies the data from a matrix A to m_name. If m_name is not initialized and the new storage format is the same or not provided, an exact copy of A is created. If already initialized, only values of the matrix elements are copied. If m_name is an allocated <i>pdcsr</i> matrix, its sparsity pattern is maintained. If the formats of A and m_name are different, the format conversion is performed. For the conversion between the <i>pdcsr</i> and <i>csr</i> formats, an intermediate matrix with the same distribution of rows on the 1D process grid as the <i>csr</i> matrix can be provided. Its sparsity is maintained during the conversion. Optional thresholding variables are used to increase the sparsity of the matrix. |                  |              |                                                                                                                                                                             |
| m_name                                                                                                                                                                                                                                                                                                                                                                                                                                                                                                                                                                                                                                                                                                                                       | input/output     | type(matrix) | The matrix where to copy                                                                                                                                                    |
| A                                                                                                                                                                                                                                                                                                                                                                                                                                                                                                                                                                                                                                                                                                                                            | input/output     | type(matrix) | The matrix to be copied                                                                                                                                                     |
| label                                                                                                                                                                                                                                                                                                                                                                                                                                                                                                                                                                                                                                                                                                                                        | input, optional  | character(5) | The storage format to use for matrix m_name                                                                                                                                 |
| threshold                                                                                                                                                                                                                                                                                                                                                                                                                                                                                                                                                                                                                                                                                                                                    | input, optional  | logical      | The tolerance for setting the elements to zero. The elements with absolute values below the threshold are omitted for the sparse formats and set to zero for the dense ones |
| threshold_is_soft                                                                                                                                                                                                                                                                                                                                                                                                                                                                                                                                                                                                                                                                                                                            | input, optional  | logical      | Whether the threshold is soft (only for dense matrices). If so, values above the threshold are shifted down to avoid discontinuity                                          |
| m_sp                                                                                                                                                                                                                                                                                                                                                                                                                                                                                                                                                                                                                                                                                                                                         | in/out, optional | type(matrix) | The intermediate matrix distributed on the 1D process grid used for the conversion to/from the <i>csr</i> format                                                            |
